# Supplementary material for: Spin- and angle-resolved inverse photoemission setup with spin orientation independent from electron incidence angle
Source: arXiv:2110.12883 source file (2022-07-21)
Supplement: Supplementary file 1 [file SupplementaryMaterial.pdf]

# Supplementary Material

## Spin- and angle-resolved inverse photoemission setup with spin orientation independent from electron incidence angle

A. F. Campos[1], P. Duret[1], S. Cabaret[1], T. Duden[2], and A. Tejeda[1]

[1]Université Paris-Saclay, CNRS, Laboratoire de Physique des Solides, 91405, Orsay, France.
[2]Constructive solutions for Science and Technology, 33649 Bielefeld, Germany.

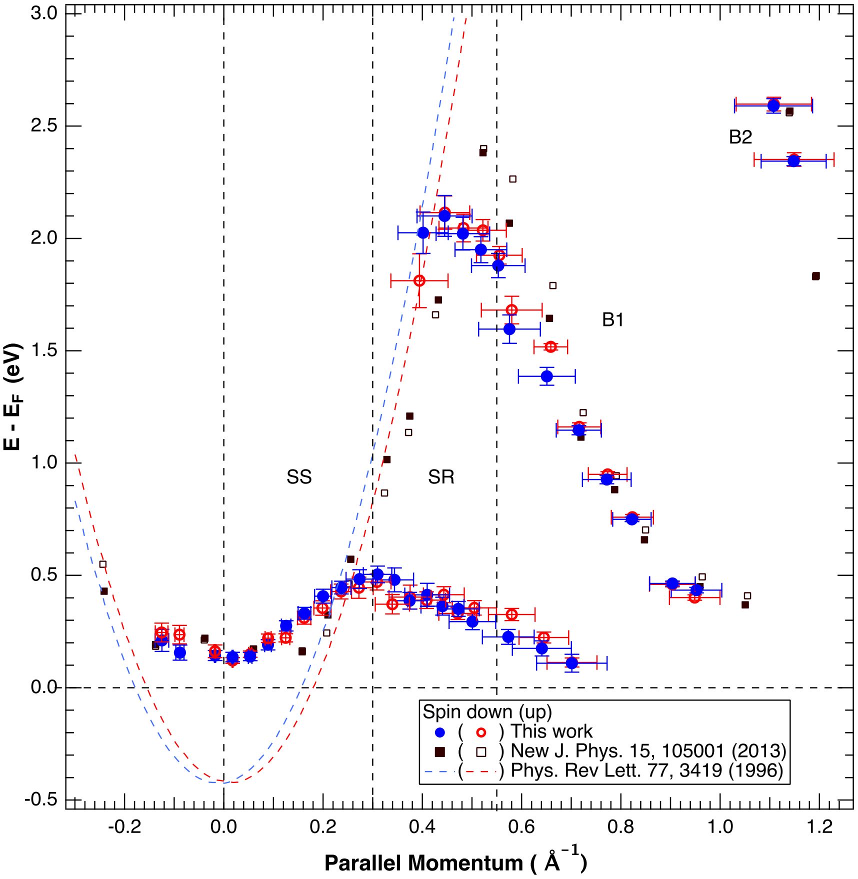


Fig. S1. Spin-polarized energy dispersion of Au(111) along the Gamma $\Gamma$M direction, derived from data in Fig. 5. Three regions are evidenced: the Shockley surface state (SS) that follows the nearly-free-electron model, the surface resonance (SR) and the bulk states (B1 and B2). Discrete values of the spin down (up) component are shown as solid (empty) circles. Reference data (squares) from S. N. Wissing, C. Eibl, A. Zumbülte, A. Schmidt, J. Braun, J. Minár, H. Ebert, and M. Donath, New Journal of Physics 15, 105001 (2013); licensed under a Creative Commons Attribution (CC BY) license. The calculated projection of the spin down (up) SS is shown as a dotted-blue (dashed-red) line (Reprinted data with permission from S. LaShell, B. McDougall, and E. Jensen, Physical Review Letters 77, 3419 (1996). Copyright 1996 by the American Physical Society).

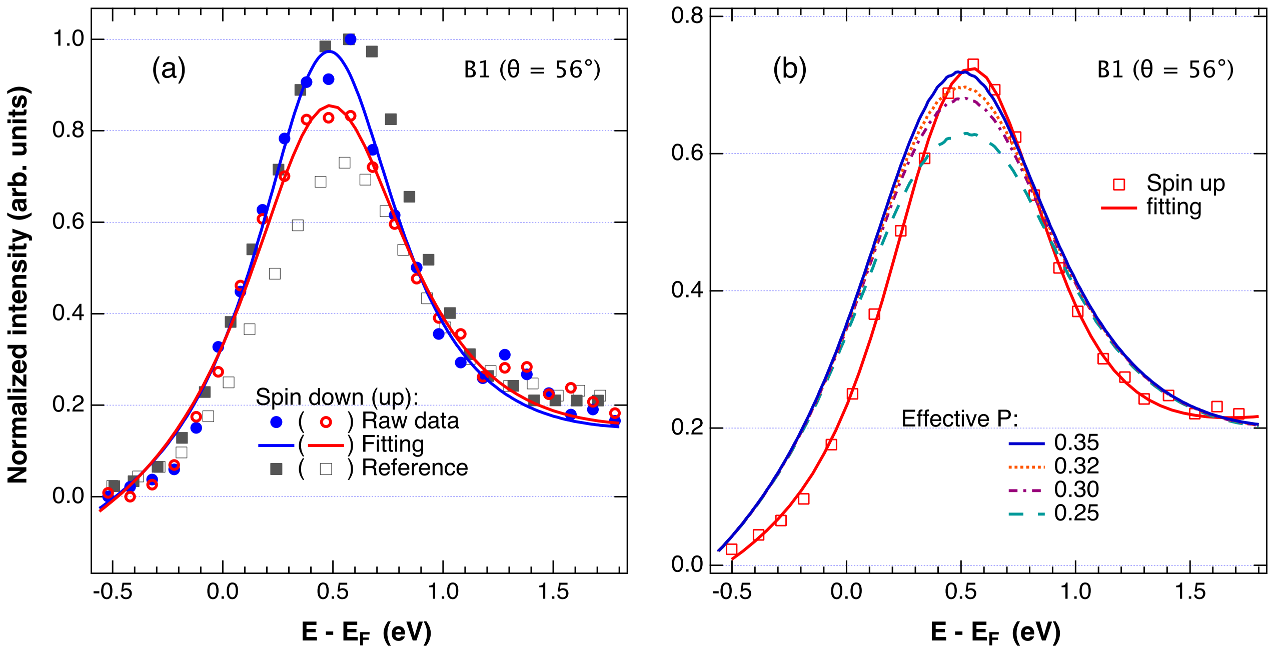


Fig. S2. (a) SPIPES spectra of Au(111) bulk state at $\theta$= 56° of our data (circles and lines). Reference data (P=0.33) (squares) from S. N. Wissing, C. Eibl, A. Zumbülte, A. Schmidt, J. Braun, J. Minár, H. Ebert, and M. Donath, New Journal of Physics 15, 105001 (2013); licensed under a Creative Commons Attribution (CC BY) license. The spin down (up) component is represented by solid (empty) markers. (b) Polarization-dependent simulations (lines) on the spin up component of reference with calibrated polarization. Our peak was simulated for different values of P by using the asymmetry function described in [Donath, M. (1989). Spin-resolved inverse photoemission of ferromagnetic surfaces. Applied Physics A, 49(4), 351-364.]. Although a perfect agreement is not expected due to different k resolutions in the setups, we estimate an effective polarization of P = 0.30 ± 0.03 for the electron source of this work.

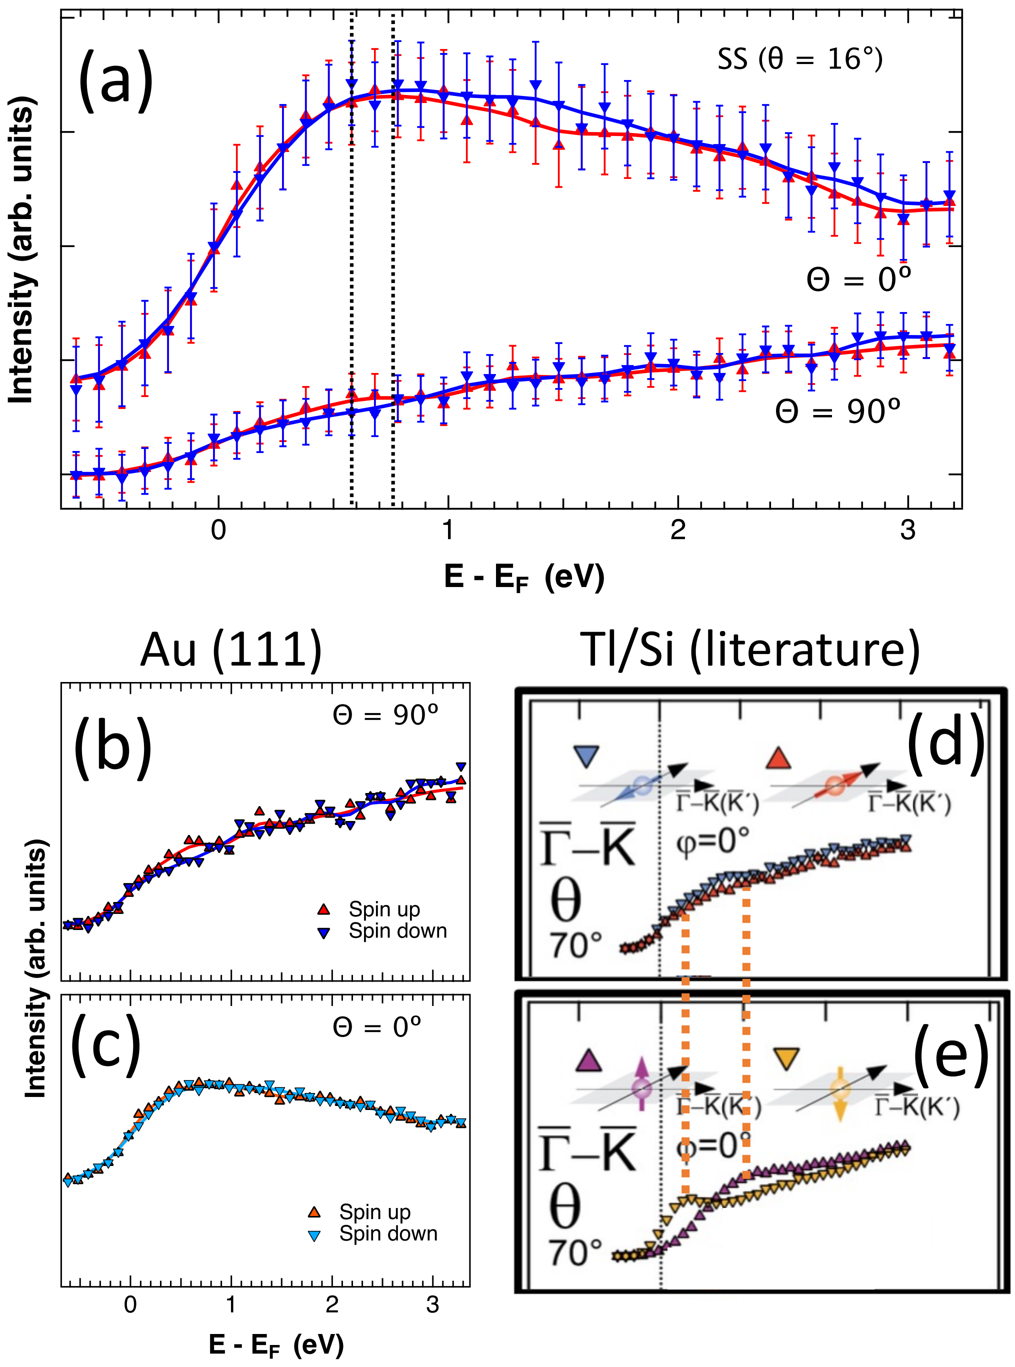


Fig. S3. (a) SPIPES spectra of Au(111) surface state at $\theta$= 16° for transversal (**Θ**=0°) and longitudinal (**Θ**=90°) spin-polarization incidences. The surface state intensity decreases for longitudinal polarization of the incoming beam. The modification of the background upon spin tuning is evident, although this has no impact for determining E(k) relationships that rely on the peak positions. (b) and (c), spectra in (a) represented to compare directly to (d) and (e), which are spectra from Tl/Si(111) for different spin-polarization incidences. The surface state intensity decreases in Tl/Si, similarly to our observations on Au(111). Reprinted figure with permission from S. Stolwijk, A. Schmidt, M. Donath, K. Sakamoto, and P. Krüger, Physical Review Letters 111, 176402 (2013). Copyright 2013 by American Physical Society.

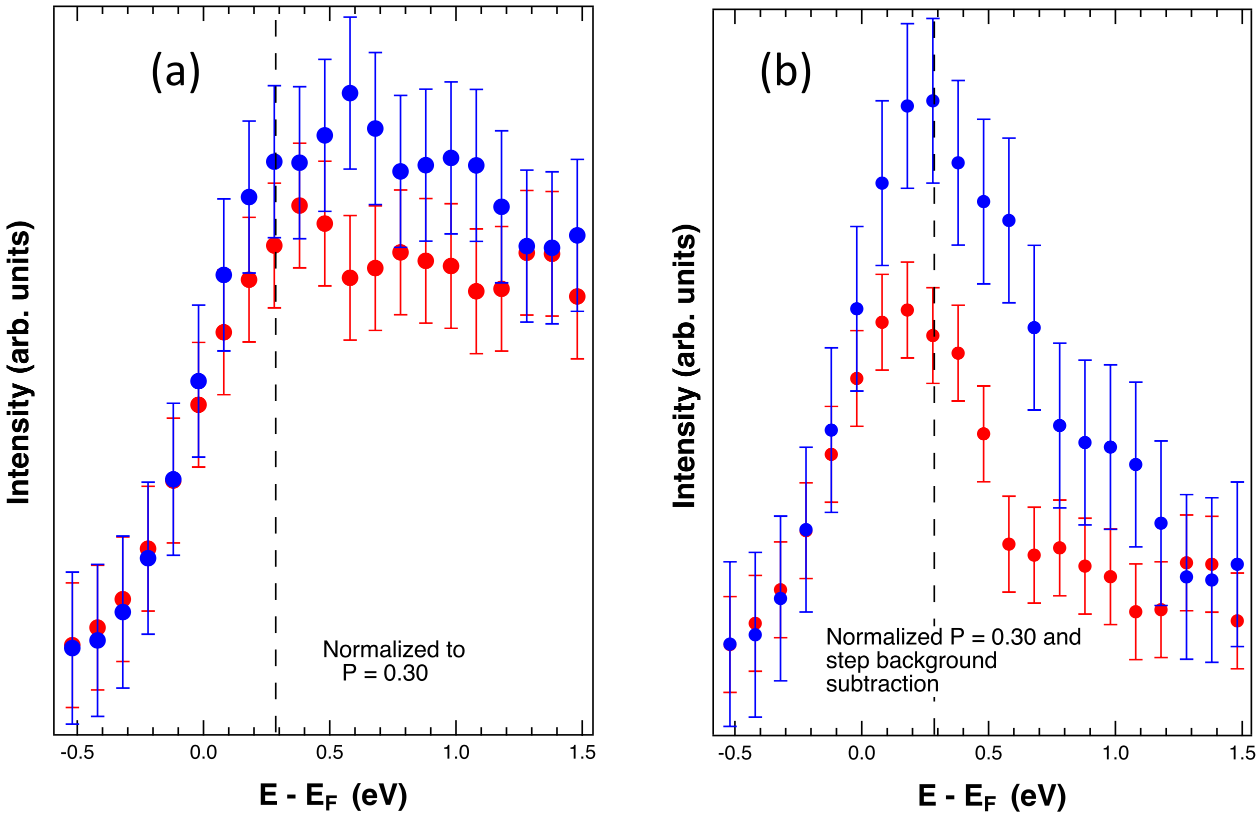


Fig. S4. Polarization normalization procedure. (a) SPIPES spectra of Au(111) surface state at $\theta$= 8° normalized to P=0.30 by using the asymmetry function described by Donath, M. Applied Physics A, 49 (4), 351-364. (b) Spectra of (a) after step background subtraction. Counting rate is about 40 Hz for the SS and data was integrated 60 seconds per point. Incident current on the sample was held below 0.8 $\mu A$.
